# Supplementary material for: NOISe: Nuclei-Aware Osteoclast Instance Segmentation for Mouse-to-Human Domain Transfer
Source: arXiv:2404.10130 source file (2024-04-15)
Supplement: Supplementary file 1 [file X_suppl.tex]

\clearpage
\setcounter{page}{1}
\maketitlesupplementary
